# Supplementary material for: Evaluation and Learning in Two-Player Symmetric Games via Best and Better Responses
Source: arXiv:2204.12791 source file (2022-04-27)
Supplement: Supplementary file 1 [file appendix.tex]

\appendix

\subsection{Proof of~\ref{lemma:se-relationship-gst-gt0}}\label{part:proof-of-se-relationship-sst}
